# Supplementary material for: ReactWorld: Structuring Interaction Responses for Embodied Video Generation
Source: arXiv:2611.06120 source file (2026-11-19)
Supplement: Supplementary file 2 [file fill_values.tex]

% Shared values for the data, implementation, and EZS-Bench results.

% Accepted source-clip duration in seconds for both AgiBot and RoVid-X.
\newcommand{\PublicClipRange}{2--13}
% S1-CHECK: Historical Web proposal settings. Verify the final batch in its launch record.
\newcommand{\WebClipRange}{2--13}
\newcommand{\WebWindow}{24}
\newcommand{\WebOverlap}{12}
\newcommand{\OutputFPS}{16}         % Video format in the main paper
\newcommand{\InterfaceBlock}{12}    % Block label in the main paper
% S1-CHECK: exported teacher field. Predicted displacement is role-conditioned.
\newcommand{\MotionMapping}{The exported $D$ uses both components of $U$ in grid-cell units. Each cell spans $16\times16$ image pixels.}
% Table S6 component scores, rounded to four decimals for display.
% Original scores are retained in the comments.
\newcommand{\VftAesthetic}{0.6054} % 0.60541000
\newcommand{\OursAesthetic}{0.6078} % 0.60777926
\newcommand{\VftImaging}{0.7520} % 0.75202593
\newcommand{\OursImaging}{0.7537} % 0.75369578
\newcommand{\VftSmoothness}{0.9560} % 0.95595216
\newcommand{\OursSmoothness}{0.9563} % 0.95628738
\newcommand{\VftBackground}{0.9031} % 0.90305867
\newcommand{\OursBackground}{0.9038} % 0.90377563
\newcommand{\VftSubject}{0.8911} % 0.89108250
\newcommand{\OursSubject}{0.8919} % 0.89188261
\newcommand{\VftOverall}{0.1315} % 0.13146651
\newcommand{\OursOverall}{0.1336} % 0.13355905
\newcommand{\VftIbg}{0.9488} % 0.94875896
\newcommand{\OursIbg}{0.9491} % 0.94914745
\newcommand{\VftIsub}{0.9434} % 0.94344528
\newcommand{\OursIsub}{0.9439} % 0.94387285
