# Supplementary material for: ReactWorld: Structuring Interaction Responses for Embodied Video Generation
Source: arXiv:2611.06120 source file (2026-11-19)
Supplement: Supplementary file 3 [file preamble.tex]

% Official CVPR 2027 fonts, margins, line numbers and title style are unchanged.
\usepackage{microtype}
\usepackage{multirow}
\definecolor{gray}{gray}{0.5}
\definecolor{cvprblue}{rgb}{0.21,0.49,0.74}
\usepackage[pagebackref,breaklinks,colorlinks,allcolors=cvprblue]{hyperref}
\hypersetup{pdftitle={ReactWorld: Supplementary Material},pdfauthor={}}
\raggedbottom
\newcommand{\FigureCaption}[2]{\captionsetup{type=figure}\caption{#1}\label{#2}}

% Queue a top float for the right column from the start of the left column.
\newcommand{\RWRightTable}[1]{%
  \suppressfloats[t]%
  \begin{table}[t]
    #1%
  \end{table}%
}
